# Supplementary material for: Trainable Highly-expressive Activation Functions
Source: arXiv:2407.07564 source file (2024-07-11)
Supplement: Supplementary file 1 [file abstract_supmat.tex]

This document contains the supplementary material for the main paper.
In \autoref{submat:toy_experiments}, we provide additional details about the regression and classification tasks in the toy-data experiments, such as data generation, training process scheme, result trends, function visualizations and further experiments.
In \autoref{submat:real_world_experiments}, we provide additional details about the training procedures of the semantic segmentation and image generation tasks in the real-world data experiments.
In \autoref{submat:ditac_versions} we present various DiTAC versions, discuss their quality, and display their illustrations.
In \autoref{submat:computational_cost} we measure DiTAC’s computational cost on various configurations.
