# Supplementary material for: Trainable Highly-expressive Activation Functions
Source: arXiv:2407.07564 source file (2024-07-11)
Supplement: Supplementary file 3 [file epoch_0_gelu_cpab.tex]

% This file was created with tikzplotlib v0.10.1.
\begin{tikzpicture}

\definecolor{darkgray176}{RGB}{176,176,176}
\definecolor{dodgerblue}{RGB}{30,144,255}

\begin{axis}[
tick align=outside,
tick pos=left,
x grid style={darkgray176},
xlabel={\(\displaystyle x\)},
xmajorgrids,
xmin=-4.4, xmax=4.4,
xtick style={color=black},
grid=both,
grid style={line width=.1pt, draw=gray!10},
major grid style={line width=.2pt,draw=gray!20},
minor x tick num=1,
minor y tick num=2,
y grid style={darkgray176},
ylabel={\(\displaystyle DiTAC(x)\)},
y label style={at={(axis description cs:-0.1,.5)},anchor=south},
ymajorgrids,
ymin=-2, ymax=4,
ytick style={color=black}
]
\addplot [semithick, dodgerblue]
table {%
-4 -0.00012671947479248
-3.91919183731079 -0.00017415032198187
-3.83838391304016 -0.000237708140048198
-3.75757575035095 -0.000322291336487979
-3.67676758766174 -0.000434250541729853
-3.59595966339111 -0.000581064610742033
-3.5151515007019 -0.000772497849538922
-3.4343433380127 -0.00102003407664597
-3.35353541374207 -0.00133783894125372
-3.27272725105286 -0.00174294819589704
-3.19191908836365 -0.00225554686039686
-3.11111116409302 -0.00289930240251124
-3.03030300140381 -0.00370162911713123
-2.9494948387146 -0.00469404365867376
-2.86868691444397 -0.0059120487421751
-2.78787875175476 -0.00739550217986107
-2.70707082748413 -0.00918773841112852
-2.62626266479492 -0.011336050927639
-2.54545450210571 -0.0138899739831686
-2.46464657783508 -0.0169011298567057
-2.38383841514587 -0.0204212907701731
-2.30303025245667 -0.0245009362697601
-2.22222232818604 -0.0291870050132275
-2.14141416549683 -0.0345202684402466
-2.06060600280762 -0.0405327528715134
-1.9797979593277 -0.0472210124135017
-1.89898991584778 -0.0543971508741379
-1.81818187236786 -0.0622401274740696
-1.73737370967865 -0.070644423365593
-1.65656566619873 -0.079422764480114
-1.57575762271881 -0.0892691761255264
-1.4949494600296 -0.100255593657494
-1.41414141654968 -0.111629031598568
-1.33333337306976 -0.123480707406998
-1.25252521038055 -0.13536325097084
-1.17171716690063 -0.147680073976517
-1.09090912342072 -0.162371888756752
-1.01010096073151 -0.177556663751602
-0.929292917251587 -0.193051502108574
-0.848484873771667 -0.20850832760334
-0.767676770687103 -0.223558127880096
-0.686868667602539 -0.239124268293381
-0.60606062412262 -0.254935622215271
-0.525252521038055 -0.27054825425148
-0.444444447755814 -0.286224842071533
-0.363636374473572 -0.301438629627228
-0.282828271389008 -0.314743041992188
-0.202020198106766 -0.325925588607788
-0.121212124824524 -0.333650529384613
-0.0404040440917015 -0.33659303188324
0.0404040440917015 -0.334809362888336
0.121212124824524 -0.325771450996399
0.202020198106766 -0.309539169073105
0.282828271389008 -0.284073263406754
0.363636374473572 -0.246581301093102
0.444444447755814 -0.202653750777245
0.525252521038055 -0.155815541744232
0.60606062412262 -0.105402044951916
0.686868667602539 -0.0543759763240814
0.767676770687103 -0.00174257659818977
0.848484873771667 0.0536900646984577
0.929292917251587 0.111103624105453
1.01010096073151 0.171802312135696
1.09090912342072 0.236998587846756
1.17171716690063 0.303542703390121
1.25252521038055 0.373682290315628
1.33333337306976 0.456345736980438
1.41414141654968 0.55264675617218
1.4949494600296 0.672233402729034
1.57575762271881 0.816165745258331
1.65656566619873 0.984010219573975
1.73737370967865 1.19043016433716
1.81818187236786 1.41387677192688
1.89898991584778 1.65011489391327
1.9797979593277 1.89577400684357
2.06060600280762 2.0200731754303
2.14141416549683 2.10689377784729
2.22222232818604 2.193035364151
2.30303025245667 2.27852916717529
2.38383841514587 2.36341714859009
2.46464657783508 2.44774556159973
2.54545450210571 2.53156447410583
2.62626266479492 2.61492657661438
2.70707082748413 2.69788289070129
2.78787875175476 2.78048324584961
2.86868691444397 2.86277484893799
2.9494948387146 2.94480085372925
3.03030300140381 3.02660131454468
3.11111116409302 3.10821175575256
3.19191908836365 3.18966341018677
3.27272725105286 3.27098441123962
3.35353541374207 3.35219764709473
3.4343433380127 3.4333233833313
3.5151515007019 3.51437902450562
3.59595966339111 3.59537863731384
3.67676758766174 3.67633318901062
3.75757575035095 3.75725340843201
3.83838391304016 3.8381462097168
3.91919183731079 3.91901755332947
4 3.99987316131592
};
\addplot [semithick, black, dashed]
table {%
-4 -4
-3.91919183731079 -3.91919183731079
-3.83838391304016 -3.83838391304016
-3.75757575035095 -3.75757575035095
-3.67676758766174 -3.67676758766174
-3.59595966339111 -3.59595966339111
-3.5151515007019 -3.5151515007019
-3.4343433380127 -3.4343433380127
-3.35353541374207 -3.35353541374207
-3.27272725105286 -3.27272725105286
-3.19191908836365 -3.19191908836365
-3.11111116409302 -3.11111116409302
-3.03030300140381 -3.03030300140381
-2.9494948387146 -2.9494948387146
-2.86868691444397 -2.86868691444397
-2.78787875175476 -2.78787875175476
-2.70707082748413 -2.70707082748413
-2.62626266479492 -2.62626266479492
-2.54545450210571 -2.54545450210571
-2.46464657783508 -2.46464657783508
-2.38383841514587 -2.38383841514587
-2.30303025245667 -2.30303025245667
-2.22222232818604 -2.22222232818604
-2.14141416549683 -2.14141416549683
-2.06060600280762 -2.06060600280762
-1.9797979593277 -1.9797979593277
-1.89898991584778 -1.89898991584778
-1.81818187236786 -1.81818187236786
-1.73737370967865 -1.73737370967865
-1.65656566619873 -1.65656566619873
-1.57575762271881 -1.57575762271881
-1.4949494600296 -1.4949494600296
-1.41414141654968 -1.41414141654968
-1.33333337306976 -1.33333337306976
-1.25252521038055 -1.25252521038055
-1.17171716690063 -1.17171716690063
-1.09090912342072 -1.09090912342072
-1.01010096073151 -1.01010096073151
-0.929292917251587 -0.929292917251587
-0.848484873771667 -0.848484873771667
-0.767676770687103 -0.767676770687103
-0.686868667602539 -0.686868667602539
-0.60606062412262 -0.60606062412262
-0.525252521038055 -0.525252521038055
-0.444444447755814 -0.444444447755814
-0.363636374473572 -0.363636374473572
-0.282828271389008 -0.282828271389008
-0.202020198106766 -0.202020198106766
-0.121212124824524 -0.121212124824524
-0.0404040440917015 -0.0404040440917015
0.0404040440917015 0.0404040440917015
0.121212124824524 0.121212124824524
0.202020198106766 0.202020198106766
0.282828271389008 0.282828271389008
0.363636374473572 0.363636374473572
0.444444447755814 0.444444447755814
0.525252521038055 0.525252521038055
0.60606062412262 0.60606062412262
0.686868667602539 0.686868667602539
0.767676770687103 0.767676770687103
0.848484873771667 0.848484873771667
0.929292917251587 0.929292917251587
1.01010096073151 1.01010096073151
1.09090912342072 1.09090912342072
1.17171716690063 1.17171716690063
1.25252521038055 1.25252521038055
1.33333337306976 1.33333337306976
1.41414141654968 1.41414141654968
1.4949494600296 1.4949494600296
1.57575762271881 1.57575762271881
1.65656566619873 1.65656566619873
1.73737370967865 1.73737370967865
1.81818187236786 1.81818187236786
1.89898991584778 1.89898991584778
1.9797979593277 1.9797979593277
2.06060600280762 2.06060600280762
2.14141416549683 2.14141416549683
2.22222232818604 2.22222232818604
2.30303025245667 2.30303025245667
2.38383841514587 2.38383841514587
2.46464657783508 2.46464657783508
2.54545450210571 2.54545450210571
2.62626266479492 2.62626266479492
2.70707082748413 2.70707082748413
2.78787875175476 2.78787875175476
2.86868691444397 2.86868691444397
2.9494948387146 2.9494948387146
3.03030300140381 3.03030300140381
3.11111116409302 3.11111116409302
3.19191908836365 3.19191908836365
3.27272725105286 3.27272725105286
3.35353541374207 3.35353541374207
3.4343433380127 3.4343433380127
3.5151515007019 3.5151515007019
3.59595966339111 3.59595966339111
3.67676758766174 3.67676758766174
3.75757575035095 3.75757575035095
3.83838391304016 3.83838391304016
3.91919183731079 3.91919183731079
4 4
};
\end{axis}

\end{tikzpicture}
