# Supplementary material for: Trainable Highly-expressive Activation Functions
Source: arXiv:2407.07564 source file (2024-07-11)
Supplement: Supplementary file 5 [file epoch_0_inf_cpab.tex]

% This file was created with tikzplotlib v0.10.1.
\begin{tikzpicture}

\definecolor{darkgray176}{RGB}{176,176,176}
\definecolor{dodgerblue}{RGB}{30,144,255}

\begin{axis}[
tick align=outside,
tick pos=left,
x grid style={darkgray176},
xlabel={\(\displaystyle x\)},
xmajorgrids,
xmin=-2, xmax=4,
xtick style={color=black},
grid=both,
grid style={line width=.1pt, draw=gray!10},
major grid style={line width=.2pt,draw=gray!20},
minor x tick num=1,
minor y tick num=2,
y grid style={darkgray176},
ylabel={\(\displaystyle inf-DiTAC(x)\)},
y label style={at={(axis description cs:-0.1,.5)},anchor=south},
ymajorgrids,
ymin=-2, ymax=4,
ytick style={color=black}
]
\addplot [semithick, dodgerblue]
table {%
-4 -4.33366441726685
-3.91919183731079 -4.24611568450928
-3.83838391304016 -4.15856695175171
-3.75757575035095 -4.07101821899414
-3.67676758766174 -3.98346924781799
-3.59595966339111 -3.89592051506042
-3.5151515007019 -3.80837178230286
-3.4343433380127 -3.72082281112671
-3.35353541374207 -3.63327431678772
-3.27272725105286 -3.54572534561157
-3.19191908836365 -3.458176612854
-3.11111116409302 -3.37062788009644
-3.03030300140381 -3.28307914733887
-2.9494948387146 -3.19553017616272
-2.86868691444397 -3.10798168182373
-2.78787875175476 -3.02043271064758
-2.70707082748413 -2.93288421630859
-2.62626266479492 -2.84533524513245
-2.54545450210571 -2.75778651237488
-2.46464657783508 -2.67023777961731
-2.38383841514587 -2.58268904685974
-2.30303025245667 -2.49514007568359
-2.22222232818604 -2.40759134292603
-2.14141416549683 -2.32004261016846
-2.06060600280762 -2.23249363899231
-1.9797979593277 -2.14494490623474
-1.89898991584778 -2.05739617347717
-1.81818187236786 -1.96984755992889
-1.73737370967865 -1.88229870796204
-1.65656566619873 -1.79474997520447
-1.57575762271881 -1.7072012424469
-1.4949494600296 -1.61965227127075
-1.41414141654968 -1.53210353851318
-1.33333337306976 -1.44455480575562
-1.25252521038055 -1.35700595378876
-1.17171716690063 -1.26945722103119
-1.09090912342072 -1.18190848827362
-1.01010096073151 -1.09435963630676
-0.929292917251587 -1.00681090354919
-0.848484873771667 -0.919262170791626
-0.767676770687103 -0.831713378429413
-0.686868667602539 -0.7441645860672
-0.60606062412262 -0.656615853309631
-0.525252521038055 -0.569067060947418
-0.444444447755814 -0.481518268585205
-0.363636374473572 -0.393969506025314
-0.282828271389008 -0.306420713663101
-0.202020198106766 -0.218871936202049
-0.121212124824524 -0.131323173642159
-0.0404040440917015 -0.0437743924558163
0.0404040440917015 0.0437743924558163
0.121212124824524 0.12454792112112
0.202020198106766 0.19039611518383
0.282828271389008 0.234271794557571
0.363636374473572 0.272235155105591
0.444444447755814 0.303788930177689
0.525252521038055 0.347768366336823
0.60606062412262 0.419402360916138
0.686868667602539 0.495249658823013
0.767676770687103 0.564208507537842
0.848484873771667 0.643500506877899
0.929292917251587 0.796203970909119
1.01010096073151 1.02991986274719
1.09090912342072 1.26927947998047
1.17171716690063 1.50863885879517
1.25252521038055 1.74799799919128
1.33333337306976 1.98735761642456
1.41414141654968 2.22671699523926
1.4949494600296 2.46607637405396
1.57575762271881 2.70543622970581
1.65656566619873 2.94479513168335
1.73737370967865 3.18415451049805
1.81818187236786 3.4235143661499
1.89898991584778 3.6628737449646
1.9797979593277 3.9022331237793
2.06060600280762 4.14159202575684
2.14141416549683 4.38095188140869
2.22222232818604 4.62031173706055
2.30303025245667 4.85967063903809
2.38383841514587 5.09903001785278
2.46464657783508 5.33838987350464
2.54545450210571 5.57774877548218
2.62626266479492 5.81710863113403
2.70707082748413 6.05646848678589
2.78787875175476 6.29582738876343
2.86868691444397 6.53518724441528
2.9494948387146 6.77454614639282
3.03030300140381 7.01390504837036
3.11111116409302 7.25326490402222
3.19191908836365 7.49262380599976
3.27272725105286 7.73198366165161
3.35353541374207 7.97134351730347
3.4343433380127 8.21070289611816
3.5151515007019 8.4500617980957
3.59595966339111 8.68942070007324
3.67676758766174 8.92878150939941
3.75757575035095 9.16814041137695
3.83838391304016 9.40749931335449
3.91919183731079 9.64685821533203
4 9.8862190246582
};
\addplot [semithick, black, dashed]
table {%
-4 -4
-3.91919183731079 -3.91919183731079
-3.83838391304016 -3.83838391304016
-3.75757575035095 -3.75757575035095
-3.67676758766174 -3.67676758766174
-3.59595966339111 -3.59595966339111
-3.5151515007019 -3.5151515007019
-3.4343433380127 -3.4343433380127
-3.35353541374207 -3.35353541374207
-3.27272725105286 -3.27272725105286
-3.19191908836365 -3.19191908836365
-3.11111116409302 -3.11111116409302
-3.03030300140381 -3.03030300140381
-2.9494948387146 -2.9494948387146
-2.86868691444397 -2.86868691444397
-2.78787875175476 -2.78787875175476
-2.70707082748413 -2.70707082748413
-2.62626266479492 -2.62626266479492
-2.54545450210571 -2.54545450210571
-2.46464657783508 -2.46464657783508
-2.38383841514587 -2.38383841514587
-2.30303025245667 -2.30303025245667
-2.22222232818604 -2.22222232818604
-2.14141416549683 -2.14141416549683
-2.06060600280762 -2.06060600280762
-1.9797979593277 -1.9797979593277
-1.89898991584778 -1.89898991584778
-1.81818187236786 -1.81818187236786
-1.73737370967865 -1.73737370967865
-1.65656566619873 -1.65656566619873
-1.57575762271881 -1.57575762271881
-1.4949494600296 -1.4949494600296
-1.41414141654968 -1.41414141654968
-1.33333337306976 -1.33333337306976
-1.25252521038055 -1.25252521038055
-1.17171716690063 -1.17171716690063
-1.09090912342072 -1.09090912342072
-1.01010096073151 -1.01010096073151
-0.929292917251587 -0.929292917251587
-0.848484873771667 -0.848484873771667
-0.767676770687103 -0.767676770687103
-0.686868667602539 -0.686868667602539
-0.60606062412262 -0.60606062412262
-0.525252521038055 -0.525252521038055
-0.444444447755814 -0.444444447755814
-0.363636374473572 -0.363636374473572
-0.282828271389008 -0.282828271389008
-0.202020198106766 -0.202020198106766
-0.121212124824524 -0.121212124824524
-0.0404040440917015 -0.0404040440917015
0.0404040440917015 0.0404040440917015
0.121212124824524 0.121212124824524
0.202020198106766 0.202020198106766
0.282828271389008 0.282828271389008
0.363636374473572 0.363636374473572
0.444444447755814 0.444444447755814
0.525252521038055 0.525252521038055
0.60606062412262 0.60606062412262
0.686868667602539 0.686868667602539
0.767676770687103 0.767676770687103
0.848484873771667 0.848484873771667
0.929292917251587 0.929292917251587
1.01010096073151 1.01010096073151
1.09090912342072 1.09090912342072
1.17171716690063 1.17171716690063
1.25252521038055 1.25252521038055
1.33333337306976 1.33333337306976
1.41414141654968 1.41414141654968
1.4949494600296 1.4949494600296
1.57575762271881 1.57575762271881
1.65656566619873 1.65656566619873
1.73737370967865 1.73737370967865
1.81818187236786 1.81818187236786
1.89898991584778 1.89898991584778
1.9797979593277 1.9797979593277
2.06060600280762 2.06060600280762
2.14141416549683 2.14141416549683
2.22222232818604 2.22222232818604
2.30303025245667 2.30303025245667
2.38383841514587 2.38383841514587
2.46464657783508 2.46464657783508
2.54545450210571 2.54545450210571
2.62626266479492 2.62626266479492
2.70707082748413 2.70707082748413
2.78787875175476 2.78787875175476
2.86868691444397 2.86868691444397
2.9494948387146 2.9494948387146
3.03030300140381 3.03030300140381
3.11111116409302 3.11111116409302
3.19191908836365 3.19191908836365
3.27272725105286 3.27272725105286
3.35353541374207 3.35353541374207
3.4343433380127 3.4343433380127
3.5151515007019 3.5151515007019
3.59595966339111 3.59595966339111
3.67676758766174 3.67676758766174
3.75757575035095 3.75757575035095
3.83838391304016 3.83838391304016
3.91919183731079 3.91919183731079
4 4
};
\end{axis}

\end{tikzpicture}
