# Supplementary material for: Trainable Highly-expressive Activation Functions
Source: arXiv:2407.07564 source file (2024-07-11)
Supplement: Supplementary file 6 [file epoch_0_leaky_cpab.tex]

% This file was created with tikzplotlib v0.10.1.
\begin{tikzpicture}

\definecolor{darkgray176}{RGB}{176,176,176}
\definecolor{dodgerblue}{RGB}{30,144,255}

\begin{axis}[
tick align=outside,
tick pos=left,
x grid style={darkgray176},
xlabel={\(\displaystyle x\)},
xmajorgrids,
xmin=-4.4, xmax=4.4,
xtick style={color=black},
grid=both,
grid style={line width=.1pt, draw=gray!10},
major grid style={line width=.2pt,draw=gray!20},
minor x tick num=1,
minor y tick num=1,
y grid style={darkgray176},
ylabel={\(\displaystyle L-DiTAC(x)\)},
y label style={at={(axis description cs:-0.1,.5)},anchor=south},
ymajorgrids,
ymin=-4.4, ymax=4.4,
ytick style={color=black}
]
\addplot [semithick, dodgerblue]
table {%
-4 -2.20000004768372
-3.91919183731079 -2.19191908836365
-3.83838391304016 -2.18383836746216
-3.75757575035095 -2.17575740814209
-3.67676758766174 -2.1676766872406
-3.59595966339111 -2.15959596633911
-3.5151515007019 -2.15151500701904
-3.4343433380127 -2.14343428611755
-3.35353541374207 -2.13535356521606
-3.27272725105286 -2.127272605896
-3.19191908836365 -2.11919188499451
-3.11111116409302 -2.11111116409302
-3.03030300140381 -2.10303020477295
-2.9494948387146 -2.09494948387146
-2.86868691444397 -2.08686876296997
-2.78787875175476 -2.0787878036499
-2.70707082748413 -2.07070708274841
-2.62626266479492 -2.06262612342834
-2.54545450210571 -2.05454540252686
-2.46464657783508 -2.04646468162537
-2.38383841514587 -2.0383837223053
-2.30303025245667 -2.03030300140381
-2.22222232818604 -2.02222228050232
-2.14141416549683 -2.01414132118225
-2.06060600280762 -2.00606060028076
-1.9797979593277 -1.97882914543152
-1.89898991584778 -1.88991177082062
-1.81818187236786 -1.80311143398285
-1.73737370967865 -1.71631121635437
-1.65656566619873 -1.62739372253418
-1.57575762271881 -1.55140566825867
-1.4949494600296 -1.48606467247009
-1.41414141654968 -1.41912996768951
-1.33333337306976 -1.35378885269165
-1.25252521038055 -1.28685426712036
-1.17171716690063 -1.2239830493927
-1.09090912342072 -1.17954432964325
-1.01010096073151 -1.13655579090118
-0.929292917251587 -1.0945907831192
-0.848484873771667 -1.05262577533722
-0.767676770687103 -1.01002311706543
-0.686868667602539 -0.971722960472107
-0.60606062412262 -0.93644654750824
-0.525252521038055 -0.902718663215637
-0.444444447755814 -0.871678233146667
-0.363636374473572 -0.841855049133301
-0.282828271389008 -0.809827923774719
-0.202020198106766 -0.776104807853699
-0.121212124824524 -0.73855459690094
-0.0404040440917015 -0.695604681968689
0.0404040440917015 -0.648711442947388
0.121212124824524 -0.594214797019958
0.202020198106766 -0.533642649650574
0.282828271389008 -0.464668750762939
0.363636374473572 -0.384121775627136
0.444444447755814 -0.301730036735535
0.525252521038055 -0.222499489784241
0.60606062412262 -0.144830226898193
0.686868667602539 -0.0721246004104614
0.767676770687103 -0.00223791599273682
0.848484873771667 0.0669522285461426
0.929292917251587 0.134894847869873
1.01010096073151 0.203611135482788
1.09090912342072 0.27483081817627
1.17171716690063 0.345191955566406
1.25252521038055 0.41761040687561
1.33333337306976 0.502147197723389
1.41414141654968 0.599829435348511
1.4949494600296 0.720865726470947
1.57575762271881 0.86599588394165
1.65656566619873 1.03449749946594
1.73737370967865 1.24153232574463
1.81818187236786 1.46442604064941
1.89898991584778 1.69901752471924
1.9797979593277 1.94211888313293
2.06060600280762 2.06060600280762
2.14141416549683 2.14141416549683
2.22222232818604 2.22222232818604
2.30303025245667 2.30303025245667
2.38383841514587 2.38383841514587
2.46464657783508 2.46464657783508
2.54545450210571 2.54545450210571
2.62626266479492 2.62626266479492
2.70707082748413 2.70707082748413
2.78787875175476 2.78787875175476
2.86868691444397 2.86868691444397
2.9494948387146 2.9494948387146
3.03030300140381 3.03030300140381
3.11111116409302 3.11111116409302
3.19191908836365 3.19191908836365
3.27272725105286 3.27272725105286
3.35353541374207 3.35353541374207
3.4343433380127 3.4343433380127
3.5151515007019 3.5151515007019
3.59595966339111 3.59595966339111
3.67676758766174 3.67676758766174
3.75757575035095 3.75757575035095
3.83838391304016 3.83838391304016
3.91919183731079 3.91919183731079
4 4
};
\addplot [semithick, black, dashed]
table {%
-4 -4
-3.91919183731079 -3.91919183731079
-3.83838391304016 -3.83838391304016
-3.75757575035095 -3.75757575035095
-3.67676758766174 -3.67676758766174
-3.59595966339111 -3.59595966339111
-3.5151515007019 -3.5151515007019
-3.4343433380127 -3.4343433380127
-3.35353541374207 -3.35353541374207
-3.27272725105286 -3.27272725105286
-3.19191908836365 -3.19191908836365
-3.11111116409302 -3.11111116409302
-3.03030300140381 -3.03030300140381
-2.9494948387146 -2.9494948387146
-2.86868691444397 -2.86868691444397
-2.78787875175476 -2.78787875175476
-2.70707082748413 -2.70707082748413
-2.62626266479492 -2.62626266479492
-2.54545450210571 -2.54545450210571
-2.46464657783508 -2.46464657783508
-2.38383841514587 -2.38383841514587
-2.30303025245667 -2.30303025245667
-2.22222232818604 -2.22222232818604
-2.14141416549683 -2.14141416549683
-2.06060600280762 -2.06060600280762
-1.9797979593277 -1.9797979593277
-1.89898991584778 -1.89898991584778
-1.81818187236786 -1.81818187236786
-1.73737370967865 -1.73737370967865
-1.65656566619873 -1.65656566619873
-1.57575762271881 -1.57575762271881
-1.4949494600296 -1.4949494600296
-1.41414141654968 -1.41414141654968
-1.33333337306976 -1.33333337306976
-1.25252521038055 -1.25252521038055
-1.17171716690063 -1.17171716690063
-1.09090912342072 -1.09090912342072
-1.01010096073151 -1.01010096073151
-0.929292917251587 -0.929292917251587
-0.848484873771667 -0.848484873771667
-0.767676770687103 -0.767676770687103
-0.686868667602539 -0.686868667602539
-0.60606062412262 -0.60606062412262
-0.525252521038055 -0.525252521038055
-0.444444447755814 -0.444444447755814
-0.363636374473572 -0.363636374473572
-0.282828271389008 -0.282828271389008
-0.202020198106766 -0.202020198106766
-0.121212124824524 -0.121212124824524
-0.0404040440917015 -0.0404040440917015
0.0404040440917015 0.0404040440917015
0.121212124824524 0.121212124824524
0.202020198106766 0.202020198106766
0.282828271389008 0.282828271389008
0.363636374473572 0.363636374473572
0.444444447755814 0.444444447755814
0.525252521038055 0.525252521038055
0.60606062412262 0.60606062412262
0.686868667602539 0.686868667602539
0.767676770687103 0.767676770687103
0.848484873771667 0.848484873771667
0.929292917251587 0.929292917251587
1.01010096073151 1.01010096073151
1.09090912342072 1.09090912342072
1.17171716690063 1.17171716690063
1.25252521038055 1.25252521038055
1.33333337306976 1.33333337306976
1.41414141654968 1.41414141654968
1.4949494600296 1.4949494600296
1.57575762271881 1.57575762271881
1.65656566619873 1.65656566619873
1.73737370967865 1.73737370967865
1.81818187236786 1.81818187236786
1.89898991584778 1.89898991584778
1.9797979593277 1.9797979593277
2.06060600280762 2.06060600280762
2.14141416549683 2.14141416549683
2.22222232818604 2.22222232818604
2.30303025245667 2.30303025245667
2.38383841514587 2.38383841514587
2.46464657783508 2.46464657783508
2.54545450210571 2.54545450210571
2.62626266479492 2.62626266479492
2.70707082748413 2.70707082748413
2.78787875175476 2.78787875175476
2.86868691444397 2.86868691444397
2.9494948387146 2.9494948387146
3.03030300140381 3.03030300140381
3.11111116409302 3.11111116409302
3.19191908836365 3.19191908836365
3.27272725105286 3.27272725105286
3.35353541374207 3.35353541374207
3.4343433380127 3.4343433380127
3.5151515007019 3.5151515007019
3.59595966339111 3.59595966339111
3.67676758766174 3.67676758766174
3.75757575035095 3.75757575035095
3.83838391304016 3.83838391304016
3.91919183731079 3.91919183731079
4 4
};
\end{axis}

\end{tikzpicture}
