# Supplementary material for: Trainable Highly-expressive Activation Functions
Source: arXiv:2407.07564 source file (2024-07-11)
Supplement: Supplementary file 7 [file epoch_0_vf.tex]

% This file was created with tikzplotlib v0.10.1.
\begin{tikzpicture}

\definecolor{chocolate}{RGB}{210,105,30}
\definecolor{darkgray176}{RGB}{176,176,176}

\begin{axis}[
tick align=outside,
tick pos=left,
x grid style={darkgray176},
xlabel={\(\displaystyle x\)},
xmajorgrids,
xmin=0, xmax=1,
xtick style={color=black},
grid=both,
grid style={line width=.1pt, draw=gray!10},
major grid style={line width=.2pt,draw=gray!20},
minor x tick num=1,
minor y tick num=1,
y grid style={darkgray176},
ylabel={\(\displaystyle v^{\btheta}(x)\)},
ymajorgrids,
ymin=-0.237489585531875, ymax=0.0194867288228124,
ytick style={color=black},
y label style={at={(axis description cs:-0.23,.5)},anchor=south},
tick label style={/pgf/number format/fixed},
]
\addplot [semithick, black, dashed]
table {%
0 0
0.0101010101010101 0
0.0202020202020202 0
0.0303030303030303 0
0.0404040404040404 0
0.0505050505050505 0
0.0606060606060606 0
0.0707070707070707 0
0.0808080808080808 0
0.0909090909090909 0
0.101010101010101 0
0.111111111111111 0
0.121212121212121 0
0.131313131313131 0
0.141414141414141 0
0.151515151515152 0
0.161616161616162 0
0.171717171717172 0
0.181818181818182 0
0.191919191919192 0
0.202020202020202 0
0.212121212121212 0
0.222222222222222 0
0.232323232323232 0
0.242424242424242 0
0.252525252525253 0
0.262626262626263 0
0.272727272727273 0
0.282828282828283 0
0.292929292929293 0
0.303030303030303 0
0.313131313131313 0
0.323232323232323 0
0.333333333333333 0
0.343434343434343 0
0.353535353535354 0
0.363636363636364 0
0.373737373737374 0
0.383838383838384 0
0.393939393939394 0
0.404040404040404 0
0.414141414141414 0
0.424242424242424 0
0.434343434343434 0
0.444444444444444 0
0.454545454545455 0
0.464646464646465 0
0.474747474747475 0
0.484848484848485 0
0.494949494949495 0
0.505050505050505 0
0.515151515151515 0
0.525252525252525 0
0.535353535353535 0
0.545454545454546 0
0.555555555555556 0
0.565656565656566 0
0.575757575757576 0
0.585858585858586 0
0.595959595959596 0
0.606060606060606 0
0.616161616161616 0
0.626262626262626 0
0.636363636363636 0
0.646464646464647 0
0.656565656565657 0
0.666666666666667 0
0.676767676767677 0
0.686868686868687 0
0.696969696969697 0
0.707070707070707 0
0.717171717171717 0
0.727272727272727 0
0.737373737373737 0
0.747474747474748 0
0.757575757575758 0
0.767676767676768 0
0.777777777777778 0
0.787878787878788 0
0.797979797979798 0
0.808080808080808 0
0.818181818181818 0
0.828282828282828 0
0.838383838383838 0
0.848484848484849 0
0.858585858585859 0
0.868686868686869 0
0.878787878787879 0
0.888888888888889 0
0.898989898989899 0
0.909090909090909 0
0.919191919191919 0
0.929292929292929 0
0.939393939393939 0
0.94949494949495 0
0.95959595959596 0
0.96969696969697 0
0.97979797979798 0
0.98989898989899 0
1 0
};
\addplot [semithick, chocolate, opacity=1.0]
table {%
0 1.06626889680535e-19
0.0101010101010101 0.000809283868875355
0.0202020202020202 0.00161856773775071
0.0303030303030303 0.00242785178124905
0.0404040404040404 0.00323713547550142
0.0505050505050505 0.00404641916975379
0.0606060606060606 0.00485570356249809
0.0707070707070707 0.00566498702391982
0.0808080808080808 0.00647427095100284
0.0909090909090909 0.00728355487808585
0.101010101010101 0.00780598726123571
0.111111111111111 0.00574668310582638
0.121212121212121 0.00368737848475575
0.131313131313131 0.00162807549349964
0.141414141414141 -0.00043122743954882
0.151515151515152 -0.00249053351581097
0.161616161616162 -0.00454983627423644
0.171717171717172 -0.0066091394983232
0.181818181818182 -0.0086684450507164
0.191919191919192 -0.0107277482748032
0.202020202020202 -0.0136815570294857
0.212121212121212 -0.0202134288847446
0.222222222222222 -0.0267452895641327
0.232323232323232 -0.0332771502435207
0.242424242424242 -0.0398090220987797
0.252525252525253 -0.0463408753275871
0.262626262626263 -0.0528727471828461
0.272727272727273 -0.059404619038105
0.282828282828283 -0.0659364685416222
0.292929292929293 -0.0724683403968811
0.303030303030303 -0.080329641699791
0.313131313131313 -0.0912928655743599
0.323232323232323 -0.102256119251251
0.333333333333333 -0.113219380378723
0.343434343434343 -0.124182604253292
0.353535353535354 -0.135145872831345
0.363636363636364 -0.146109119057655
0.373737373737374 -0.157072350382805
0.383838383838384 -0.168035611510277
0.393939393939394 -0.178998872637749
0.404040404040404 -0.185800477862358
0.414141414141414 -0.186359703540802
0.424242424242424 -0.186918914318085
0.434343434343434 -0.187478125095367
0.444444444444444 -0.188037350773811
0.454545454545455 -0.188596561551094
0.464646464646465 -0.189155787229538
0.474747474747475 -0.189714998006821
0.484848484848485 -0.190274208784103
0.494949494949495 -0.190833434462547
0.505050505050505 -0.190527930855751
0.515151515151515 -0.18935763835907
0.525252525252525 -0.188187345862389
0.535353535353535 -0.187017053365707
0.545454545454546 -0.185846775770187
0.555555555555556 -0.184676483273506
0.565656565656566 -0.183506190776825
0.575757575757576 -0.182335913181305
0.585858585858586 -0.181165620684624
0.595959595959596 -0.179995328187943
0.606060606060606 -0.182419791817665
0.616161616161616 -0.187240794301033
0.626262626262626 -0.19206178188324
0.636363636363636 -0.196882799267769
0.646464646464647 -0.201703801751137
0.656565656565657 -0.206524819135666
0.666666666666667 -0.211345836520195
0.676767676767677 -0.216166839003563
0.686868686868687 -0.22098782658577
0.696969696969697 -0.225808843970299
0.707070707070707 -0.225560307502747
0.717171717171717 -0.223139062523842
0.727272727272727 -0.220717802643776
0.737373737373737 -0.218296572566032
0.747474747474748 -0.215875327587128
0.757575757575758 -0.213454082608223
0.767676767676768 -0.211032837629318
0.777777777777778 -0.208611577749252
0.787878787878788 -0.206190332770348
0.797979797979798 -0.203769102692604
0.808080808080808 -0.195632606744766
0.818181818181818 -0.18606735765934
0.828282828282828 -0.176502093672752
0.838383838383838 -0.166936844587326
0.848484848484849 -0.1573715955019
0.858585858585859 -0.147806391119957
0.868686868686869 -0.138241142034531
0.878787878787879 -0.128675878047943
0.888888888888889 -0.119110628962517
0.898989898989899 -0.10954537987709
0.909090909090909 -0.0987171828746796
0.919191919191919 -0.0877486541867256
0.929292929292929 -0.0767800658941269
0.939393939393939 -0.0658114776015282
0.94949494949495 -0.0548428855836391
0.95959595959596 -0.0438742972910404
0.96969696969697 -0.0329057052731514
0.97979797979798 -0.0219371803104877
0.98989898989899 -0.0109685901552439
1 0
};
\end{axis}

\end{tikzpicture}
